# Supplementary material for: Binary Radiance Fields
Source: arXiv:2306.07581 source file (2023-12-04)
Supplement: Supplementary file 1 [file ablation.tex]

\section{Additional Ablation Study}
