# Supplementary material for: Binary Radiance Fields
Source: arXiv:2306.07581 source file (2023-12-04)
Supplement: Supplementary file 2 [file nerf_synthetic_ssim.tex]

\begin{table*}[!ht]
    \centering
    \caption{Quantitative results of model size and reconstruction quality (SSIM) on the Synthetic-NeRF dataset.}
    \resizebox{\textwidth}{!}{
    \begin{tabular}{L{3.5cm}P{1cm}P{1cm}P{1cm}P{1cm}P{1cm}P{1cm}P{1cm}P{1cm}P{1cm}}
    \toprule
    Method & \textit{chair} & \textit{drums} & \textit{ficus} & \textit{hotdog} & \textit{lego} & \textit{materials} & \textit{mic} & \textit{ship} & Avg. \\
    \midrule
    DVGO & 0.977 & 0.930 & 0.978 & 0.980 & 0.977 & 0.950 & 0.983 & 0.878 & 0.956 \\
    Plenoxels & 0.977 & 0.933 & 0.976 & 0.980 & 0.975 & 0.949 & 0.985 & 0.890 & 0.958 \\
    TensoRF-CP & 0.976 & 0.922 & 0.965 & 0.975 & 0.972 & \cellcolor{red!50} 0.950 & 0.983 & 0.856 & 0.950 \\
    TensoRF-VM & \cellcolor{orange!50} 0.985 & \cellcolor{orange!50} 0.936 & \cellcolor{yellow!50} 0.983 & \cellcolor{red!50} 0.983 & \cellcolor{red!50} 0.983 & \cellcolor{orange!50} 0.952 & 0.988 & \cellcolor{red!50} 0.895 & 0.963 \\
    CCNeRF-CP & 0.941 & 0.902 & 0.952 & 0.956 & 0.944 & 0.927 & 0.969 & 0.826 & 0.927 \\
    CCNeRF-HY & 0.977 & 0.920 & 0.962 & 0.975 & 0.969 & 0.934 & 0.984 & 0.855 & 0.947 \\
    Instant-NGP & 0.979 & 0.931 & 0.968 & 0.984 & 0.979 & 0.946 & 0.984 & 0.895 & 0.958 \\
    K-Planes-explicit & 0.983 & 0.938 & 0.975 & 0.981 & 0.982 & 0.948 & 0.988 & \cellcolor{yellow!50} 0.896 & 0.961 \\
    K-Planes-hybrid & 0.983 & 0.938 & 0.975 & 0.981 & 0.982 & 0.948 & 0.988 & \cellcolor{orange!50} 0.896 & 0.961 \\
    \midrule
    Ours-F1 & 0.973 & 0.921 & 0.974 & 0.973 & 0.965 & 0.934 & 0.985 & 0.877 & 0.950 \\
    Ours-F2 & 0.980 & 0.930 & 0.981 & 0.978 & 0.976 & 0.943 & \cellcolor{yellow!50} 0.989 & 0.888 & 0.958 \\
    Ours-F4 & \cellcolor{yellow!50} 0.984 & \cellcolor{yellow!50} 0.934 & \cellcolor{orange!50} 0.983 & \cellcolor{yellow!50} 0.980 & \cellcolor{yellow!50} 0.980 & 0.948 & \cellcolor{orange!50} 0.991 & 0.895 & 0.962 \\
    Ours-F8 & \cellcolor{red!50} 0.986 & \cellcolor{red!50} 0.937 & \cellcolor{red!50} 0.984 & \cellcolor{orange!50} 0.981 & \cellcolor{orange!50} 0.982 & \cellcolor{yellow!50} 0.951 & \cellcolor{red!50} 0.992 & 0.897 & 0.964 \\
    \bottomrule
    \end{tabular}}
    \label{tab:nerf_synthetic_psnr}
\end{table*}
